# Supplementary material for: AutoDAN: Generating Stealthy Jailbreak Prompts on Aligned Large Language Models
Source: arXiv:2310.04451 source file (2024-03-20)
Supplement: Supplementary file 1 [file 10-Rebuttal-STD.tex]

\section{Standard Error of Improvement}\label{standard_error}
In Tables~\ref{tab_effective_no_defense} and~\ref{tab_transfer}, the results show that both Vicuna-7b and Guanaco-7b are not very robust (attacks can achieve 97+\% ASR on them), leading to the improvement of AutoDan-HGA compared with AutoDAN-GA become implicit. However, in robust LLM like Llama2, AutoDan-HGA has explicit improvement compared with AutoDAN-GA, as the optimization based on this model becomes challenging. Specifically, we share the ablation study Table~\ref{tab_ablation}, AutoDan-HGA surpasses AutoDan-GA by 8\% in attack effectiveness and also lowers the computational cost.

The aforementioned results are gained from the scalable dataset (AdvBench Behaviour) that can guarantee reliability. In addition, we conducted a study on the standard error, based on the Llama2 and 100 data pairs from the AdvBench Behaviour dataset. The study on AutoDAN involves 5 random runs. The results are as follows:

\begin{table}[h]
\centering
\caption{Attack performance on multiple random runs}
\vspace{-0.1cm}
\label{std_table}%
    \begin{small}\resizebox{.7\linewidth}{!}{%
    \begin{tabular}{ccc}
    \toprule
    Metric & Avg. Keyword ASR (standard error) (improvement) & Avg. Time Cost (standard error) (improvement) \\
    \midrule
    GCG   & 0.44 (no std) (+0\%) & 920.0s (no std) (+0\%) \\
    AutoDAN-GA & 0.51 (0.006) (+15.9\%) & 752.6s (37.622) (-18.2\%) \\
    AutoDAN-HGA & 0.584 (0.005) (+32.7\%) & 679.6s (36.838) (-26.1\%) \\
    \bottomrule
    \end{tabular}%
}
\end{small}
\vspace{-0.2cm}
\end{table}%

The above results validate that both methods have improvement compared with GCG, and AutoDAN-HGA has improvement compared with AutoDAN-GA.
