# Supplementary material for: AutoDAN: Generating Stealthy Jailbreak Prompts on Aligned Large Language Models
Source: arXiv:2310.04451 source file (2024-03-20)
Supplement: Supplementary file 2 [file 6-Rebuttal-Init.tex]

\section{Ablations Studies on the Initial Prompts}\label{ablation_init}
Due to the nature of the genetic algorithm, its effectiveness has to rely on the initial samples which decide the initial searching space of the algorithm. However, in this paper, we argue that, since there exist many handcrafted jailbreak prompts found by the community (more than automatic methods), we can utilize them as excellent initial samples. So, finding a qualified prototype prompt is not hard. We also conduct experiments to evaluate AutoDAN under different prototype prompts. We select additional three types of prototype prompts (named AIM, SDA, UCAR) from \url{https://www.jailbreakchat.com}. We randomly select 100 data pairs from AdvBench and select the LLama2 as our targeted attack model. The results are as follows:

\begin{table}[h]
\centering
\caption{The attack performance of AutoDAN-GA on different prototype jailbreak prompts}
\vspace{-0.1cm}
\label{different_init}%
    \begin{small}\resizebox{.7\linewidth}{!}{%
    \begin{tabular}{ccccc}
    \toprule
    Prototypes & Dev Mode ( it used in our original paper) & AIM   & SDA   & UCAR \\
    \midrule
    ASR before AutoDAN’s optimization & 0.02  & 0.02  & 0.01  & 0.02  \\
    ASR after AutoDAN’s optimization & 0.51  & 0.45  & 0.49  & 0.56  \\
    \bottomrule
    \end{tabular}%
}
\end{small}
\vspace{-0.2cm}
\end{table}%

From Tab.~\ref{different_init}, we can observe that none of the prototype jailbreak prompts can achieve an ASR higher than 0.02 before being optimized by AutoDAN. From the results, we can draw the conclusion that the optimization process of AutoDAN matters: AutoDAN can improve all attack effectiveness by a large margin regardless of the prototype jailbreak prompt.
